# Supplementary material for: Flavor symmetry breaking in spin-orbit coupled bilayer graphene
Source: arXiv:2302.12284 source file (2023-06-21)
Supplement: Supplementary file 1 [file BLG_FSB_SM.pdf]

# Supplemental Material for “Flavor symmetry breaking in spin-orbit coupled bilayer graphene”

Ming Xie and Sankar Das Sarma  
*Condensed Matter Theory Center and Joint Quantum Institute, Department of Physics,  
University of Maryland, College Park, Maryland 20742, USA*

## I. BILAYER GRAPHENE EFFECTIVE NON-INTERACTING HAMILTONIAN

The electronic structure of Bernal-stacked bilayer graphene features four  $\pi$  bands formed from the  $p_z$  orbitals on the A and B sublattices of the two layers. The dispersion near the Brillouin zone corners,  $+K$  and  $-K$  valleys, can be accurately captured by the expansion of the effective tight binding model to linear order in momentum<sup>1</sup>. The Hamiltonian in the layer ( $l = 1, 2$ ) and sublattice ( $\sigma = A, B$ ) basis  $\{A1, B1, A2, B2\}$  writes:

$$\mathcal{H}_{0,\tau}(\mathbf{k}) = \begin{pmatrix} -D/2 & v_0\pi^\dagger & -v_4\pi^\dagger & v_3\pi \\ v_0\pi & -D/2 + \delta & t_1 & -v_4\pi^\dagger \\ -v_4\pi & t_1 & D/2 + \delta & v_0\pi^\dagger \\ -v_3\pi^\dagger & -v_4\pi & v_0\pi & D/2 \end{pmatrix}, \quad (\text{S1})$$

where  $\pi^\dagger = (\tau k_x - i k_y)a$  and  $\tau = \pm$  represents  $\pm K$  valley.  $a$  is the lattice constant.  $D$  is the interlayer potential generated by applied external electric field perpendicular to the layer plane.  $v_0 = 2261$  meV is the Dirac velocity given by the intralayer nearest neighbor hopping.  $\delta = 15$  meV is the mutual on-site potential between bottom layer  $B1$  and top layer  $A2$  atoms which are overlapping vertically.  $t_1 = 361$  meV is the interlayer hopping between the  $B1$  and  $A2$  sites.  $v_3 = 245$  meV and  $v_4 = 120$  meV correspond to interlayer next-nearest and third-nearest hoppings, and are dispersive because of the change in-plane coordinate during hopping. Fig. S1 plots typical electronic structure of bilayer graphene (in the absence of spin-orbit coupling and external in-plane magnetic field.)

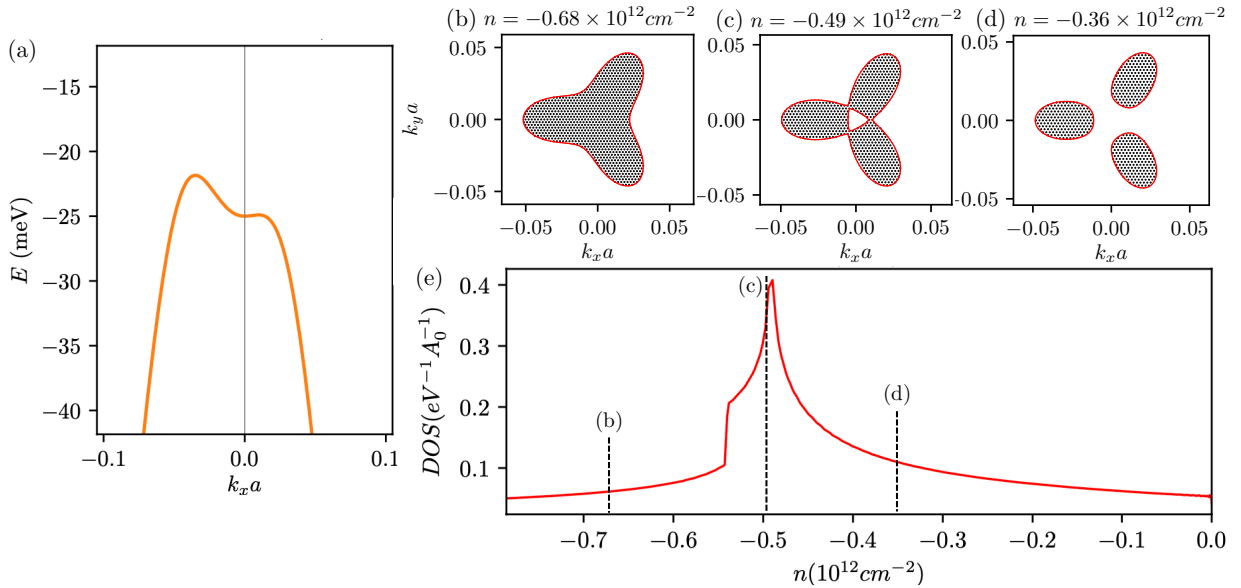

FIG. S1: (a) Dispersion of the highest valence band along  $k_x$  direction at  $U = 50$  meV. (b-d) Fermi surfaces at different densities  $n = -0.68 \times 10^{12} \text{ cm}^{-2}$ ,  $-0.49 \times 10^{12} \text{ cm}^{-2}$ , and  $-0.36 \times 10^{12} \text{ cm}^{-2}$ , with distinct Fermi surface topology. The black dots mark the filled momentum grid. (e) Density of states as a function total density.  $A_0$  is the unit cell area.

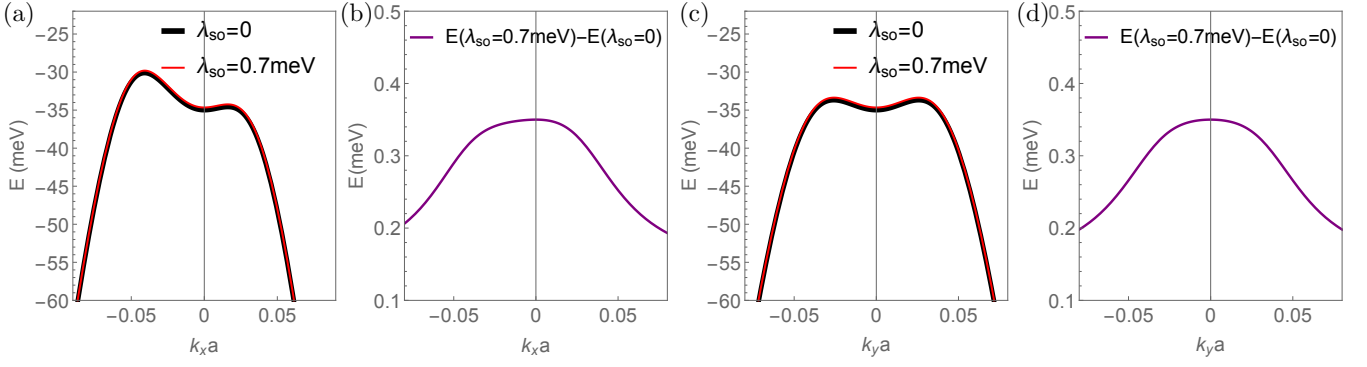

FIG. S2: Bilayer graphene bandstructure with proximity induced Ising SOC. (a) Dispersion of the highest valence band along  $k_x$  direction for  $\lambda_{so} = 0$  (black) and  $\lambda_{so} = 0.4$  meV (red). (b) Difference in band dispersions shown in (a) between  $\lambda_{so} = 0.2$  meV and  $\lambda_{so} = 0$  along  $k_x$  direction. (c-d) Same as (a-b) along  $k_y$  direction. The bands are plotted for the  $+K, \uparrow$  flavor as an example.

## II. ISING SPIN-ORBIT COUPLING

Placing bilayer graphene on top of a WSe<sub>2</sub> substrate induces spin-orbit coupling (SOC) effect in the layer closest to the WSe<sub>2</sub>. Here we focus on the Ising SOC which is the dominant effect. The Ising SOC Hamiltonian is given by:

$$H_{so} = \lambda_{so} \tau_z s_z P_{l=1} \quad (S2)$$

where  $\lambda_{so}$  is the SOC strength.  $\tau_z$ ,  $s_z$  and  $l_z$  are Pauli matrices in valley, spin and layer degrees of freedom respectively.  $P_{l=1}$  projects to the bottom layer ( $l = 1$ ). For positive interlayer potential  $D > 0$ , states near the top (bottom) of the valence (conduction) band is localized on the bottom (top) layer; therefore, the Ising SOC mainly acts on the valence band states.

The dispersion of the highest valence band with Ising SOC is shown in Fig. S2 for a typical value  $\lambda_{so} \sim 0.7$  meV close to the value extracted from experiment<sup>2</sup>. The electron wavefunction is layer polarized near  $k = 0$ . As  $\mathbf{k}$  deviates away from 0, the layer polarization reduces and the electron wavefunction evolves towards having equal weight on both layers. Because of this change in the wavefunction, the split in band dispersion gradually decreases as the momentum increases.

## III. ORBITAL EFFECT OF IN-PLANE MAGNETIC FIELD

When an in-plane magnetic field is applied parallel to the graphene bilayer, it induces both orbital and Zeeman effects on the electronic structure. The orbital effect originates from the difference in the vector potential at the two layers. In the symmetric gauge, the vector potential  $\mathbf{A} = z(B_y, -B_x, 0)$  for a magnetic field  $\mathbf{B} = (B_x, B_y, 0)$ . The vertical coordinate for the bottom (top) layer is  $z_1 = -d_0/2$  ( $z_2 = d_0/2$ ) where  $d_0$  is the interlayer spacing. The vector potential enters as a phase in the intralayer hopping integral. When expanded near the  $\pm K$  point, the Hamiltonian becomes

$$\mathcal{H}_{0,\tau}(\mathbf{k}) = \begin{pmatrix} -D/2 & v_0 \pi_1^\dagger & -v_4 \pi^\dagger & v_3 \pi \\ v_0 \pi_1 & -D/2 + \delta & t_1 & -v_4 \pi^\dagger \\ -v_4 \pi & t_1 & D/2 + \delta & v_0 \pi_2^\dagger \\ -v_3 \pi^\dagger & -v_4 \pi & v_0 \pi_2 & D/2 \end{pmatrix}, \quad (S3)$$

where  $\pi_l = \tau(k_x + eA_{l,x}/\hbar)a + i(k_y + eA_{l,y}/\hbar)a$  with  $\mathbf{A}_l = \mathbf{A}|_{z=z_l}$ . The interlayer distance  $d_0 = 3.3\text{\AA}$ . For a magnetic field  $B = 1$  T, the magnitude of the momentum shift  $e|\mathbf{A}|a/\hbar = 6.26 \times 10^{-5}$ , which is three orders of magnitude smaller than the typical Fermi surface dimension  $k_F a \sim 10^{-2}$ . Therefore, we expect the orbital effect induced by in-plane magnetic field has negligible modification to the band dispersion and Fermi surface geometry near band edges.

Figure S3 compares the band dispersions with and without the orbital effect. Because the orbital effect modification is identical for all the four flavors (related by time reversal symmetry), it has little effect on the flavor symmetry

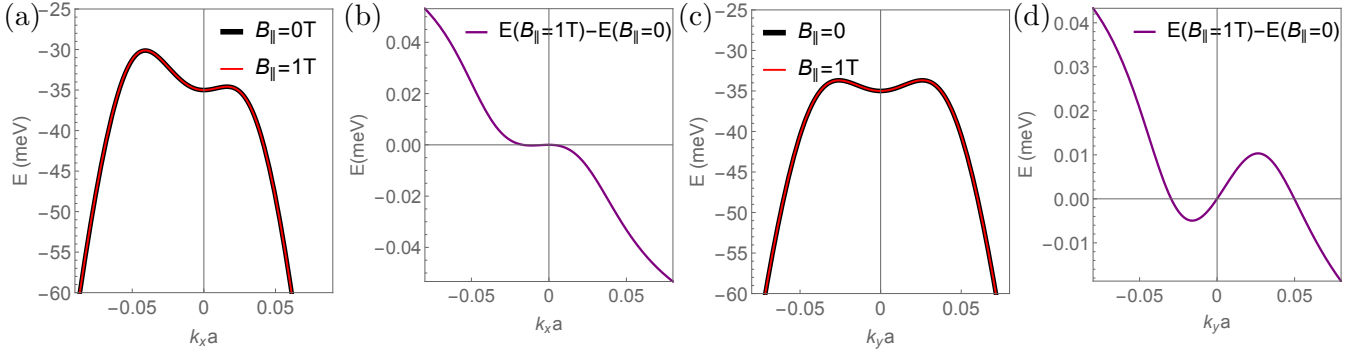

FIG. S3: Bilayer graphene bandstructure under in-plane magnetic field. (a) Dispersion of the highest valence band along  $k_x$  direction for  $B = 0$  (black) and  $B = 1$  T (red). (b) Difference in energy dispersion between  $B = 1$  T and  $B = 0$ . (c-d) Same as (a-b) along  $k_y$  direction. We have assumed  $\mathbf{B}$  along  $x$ -direction as an example.

breaking transition. In contrast, the Zeeman field,  $E_Z \approx 0.12$  meV for  $B = 1$  T, directly changes the energy of different flavor orderings and is the dominant term in our theory.

#### IV. MEAN-FIELD GROUND STATES UNDER IN-PLANE MAGNETIC FIELD

The in-plane magnetic field generates Zeeman spin splitting which introduces a spin-quantization axis along the direction of the magnetic field. It breaks the  $SU(2)_+ \times SU(2)_-$  symmetry of the interacting BLG Hamiltonian. If one defines the positive direction of spin to be opposite in the two valleys, the Zeeman effect Hamiltonian can be written in the form

$$H_Z = \frac{1}{2} E_Z \tau_z s_z, \quad (\text{S4})$$

which is similar to the Ising SOC ignoring the layer degree of freedom. The magnitude of the Zeeman splitting needed for the observation of superconductivity is about 0.1 meV for a field  $B \sim 1$  T<sup>3</sup>. Because of this, we predict that the flavor symmetry breaking phase diagram under in-plane magnetic field is qualitatively the same as that in Fig. 4 of the main text. Our numerical calculation using Eq. S4 also verifies this prediction. This also shows the effect of decreasing layer polarization when  $\mathbf{k}$  moves away from 0 is negligible in the Ising SOC.

| Phases | $E_Z = 0$                                                                                           | $E_Z > 0$                                                                         |
|--------|-----------------------------------------------------------------------------------------------------|-----------------------------------------------------------------------------------|
| SVP1   | $\mathcal{R}_+  +\uparrow\rangle\langle+\uparrow  \mathcal{R}_+^{-1}$                               | $ +\downarrow\rangle\langle+\downarrow $                                          |
| IVC-SP | $\mathcal{R}_+  +\uparrow\rangle\langle-\uparrow  \mathcal{R}_+^{-1}$                               | $ +\downarrow\rangle\langle-\downarrow $                                          |
| SP     | $\sum_{\tau} \mathcal{R}_{\tau}  \tau\uparrow\rangle\langle\tau\uparrow  \mathcal{R}_{\tau}^{-1}/2$ | $( +\downarrow\rangle\langle+\downarrow  +  -\uparrow\rangle\langle-\uparrow )/2$ |
| IVC    | $\sum_s \mathcal{R}_s  +\uparrow s\rangle\langle-\uparrow s  \mathcal{R}_s^{-1}/2$                  | $( +\uparrow\rangle\langle-\downarrow  +  +\downarrow\rangle\langle-\uparrow )/2$ |
| SVP3   | $(I - \mathcal{R}_+  +\uparrow\rangle\langle+\uparrow  \mathcal{R}_+^{-1})/3$                       | $(I -  +\uparrow\rangle\langle+\uparrow )/3$                                      |

TABLE S1: Flavor configurations for different symmetry breaking phases in the absence ( $B_Z = 0$ ) and presence ( $B_Z > 0$ ) of the in-plane magnetic field. For flavor polarized phases, the table element represents the valley diagonal component of the density matrix; for intervalley coherent phases it represents valley off-diagonal component of the density matrix.  $\mathcal{R}_{\pm}$  indicates spin rotation degeneracy of the ground states.

The flavor configurations for the ground states under in-plane magnetic field are different compared to the Ising SOC case. In the normal basis where positive spin direction is the same for both valleys, the flavor configurations are listed in Table S1. It can be obtained simply from Table 1 in the main text by reversing the spin in the  $-K$  valley (for  $E_Z > 0$ ).

#### V. EXTENDED FLAVOR SYMMETRY BREAKING PHASE DIAGRAMS

In this section, we show extended numerical results on the flavor symmetry breaking phase diagram. In particular, the phase diagrams as a function of  $n$  and  $D$  with different gate distance  $d$  and SOC strength  $\lambda_{so}$  are shown in Fig.

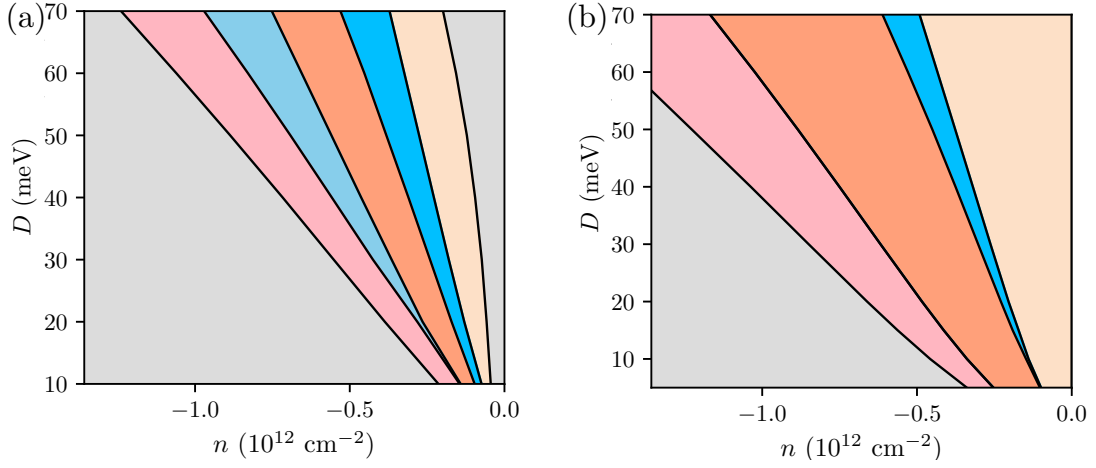

FIG. S4: Flavor symmetry breaking phase diagram for (a) small gate distance  $d = 5$  nm with fixed  $\epsilon = 10$  and  $\lambda_{so} = 0$ , and (b) strong Ising SOC  $\lambda_{so} = 1.0$  meV with fixed  $d = 30$  nm and  $\epsilon = 10$ .

S4. When the metallic gates is closer to the graphene bilayer, the paramagnetic (PM) phase also appears near zero density  $n \sim 0$  in addition to the high density limit. In general, the Fermi surface topology becomes subtle when screening effect is strong, i.e., for small  $d$  and/or large  $\epsilon$ .

Figure S5 shows the  $\lambda_{so}$ - $n$  phase diagram at two different bias voltages  $D = 20$  meV and  $D = 60$  meV. The SP/IVC-SP and the IVC-SP/SVP1 phase boundaries remain nearly independent of  $\lambda_{so}$ .

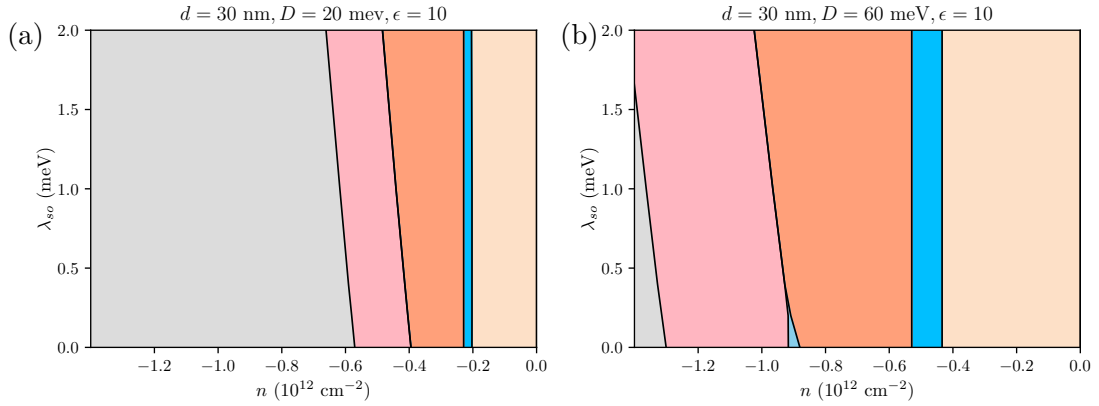

FIG. S5: Flavor symmetry breaking phase diagram in the presence of Ising SOC  $\lambda_{so} = 0$  at different interlayer electric potential (a)  $D = 20$  meV and (b)  $D = 60$  meV. In both cases, we have set  $d = 30$  nm and  $\epsilon = 10$ .

<sup>1</sup> J. Jung and A. H. MacDonald, Phys. Rev. B **89**, 035405 (2014).

<sup>2</sup> Y. Zhang, R. Polski, A. Thomson, E. Lantagne-Hurtubise, C. Lewandowski, H. Zhou, K. Watanabe, T. Taniguchi, J. Alicea, and S. Nadj-Perge, Nature **613**, 268 (2023).

<sup>3</sup> H. Zhou, L. Holleis, Y. Saito, L. Cohen, W. Huynh, C. L. Patterson, F. Yang, T. Taniguchi, K. Watanabe, and A. F. Young, Science **375**, 774 (2022).
